# Supplementary material for: Automated LTL Specification Generation from Industrial Aerospace Requirements
Source: arXiv:2604.21715 source file (2026-04-21)
Supplement: Supplementary file 1 [file Appendix.tex]

%%%%%%%%%%%%%%%%%%%%%%%%%%% Data Availability
%\vspace{-5pt}
\subsection{Data Availability} \label{sec:dataavil}
%\vspace{-2.5pt}

To facilitate future research and ensure reproducibility, we provide a comprehensive reproduction package. The package includes: (1) the autospec tool (source code) and pre-configured Docker images; (2) the complete evaluation datasets, including the X.509 case study and other benchmarks; (3) raw verification logs and proof reports; and (4) experimental scripts for automated batch execution. Regarding system requirements, the artifact can be evaluated on any standard x86-64 machine with Docker installed, eliminating the need for specific OS versions (\eg, Ubuntu 18.04) or complex environment setup.

%\vspace{-5pt}
\subsubsection{Artifact Check-List (Meta-Infomation)}
%\vspace{-2.5pt}

\begin{itemize}[nosep]
    \setlength{\baselineskip}{13.5pt}
    \item \emph{Dataset:} A list of download addresses for evaluation datasets with a specific version or commit ID.
    \item \emph{Run-time environment:} Linux.
    \item \emph{Hardware:} X86.
    \item \emph{How much disk space is required (approximately)?:} 50 MB for our code package and an additional 6 GB for docker images.
    \item \emph{Publicly available?:} Yes.
    \item \emph{Code licenses (if publicly available)?:} MIT.
    \item \emph{Archived (provide DOI)?:} Yes.
\end{itemize}

%\vspace{-5pt}
\subsubsection{Description}
%\vspace{-2.5pt}

\begin{itemize}[nosep]
    \setlength{\baselineskip}{13.5pt}
    \item \emph{How to access:}
        \begin{itemize}[nosep]
        \setlength{\baselineskip}{13.5pt}
            \item The reproducible artifact can be downloaded from the following link: \url{https://sites.google.com/view/autospecification}.
            \item The source code, deployment guide, and raw experimental data are publicly available on GitHub: \url{https://github.com/Xidian-ICTT-GZ/AutoSpec}.
        \end{itemize}
        
    \item \emph{Hardware dependencies:} Any standard machine capable of running Docker (x86-64 recommended, but ARM/Apple Silicon is supported via emulation). An \textbf{active internet connection} is required to access remote LLM APIs.
    
    \item \emph{Software dependencies:} 
        \begin{itemize}[nosep]
        \setlength{\baselineskip}{13.5pt}
            \item \textbf{Docker Engine} (or Docker Desktop) is the only requirement for the host system.
            \item All tool-specific dependencies (\eg, \framac, Clang, Python libraries) are fully encapsulated within the provided Docker image.
        \end{itemize}        
\end{itemize}

%\vspace{-5pt}
\subsubsection{Installation}
%\vspace{-2.5pt}

\begin{itemize}[nosep]
    \setlength{\baselineskip}{13.5pt}
    \item Please refer to the \texttt{README.md} file in the artifact or GitHub repository.
\end{itemize}

%%%%%%%%%%%%%%%%%%%%%%%%%%% Additional Experimental Information
\subsection{Additional Experimental Information} \label{sec:exper}

\input{Table/Table1}
\begin{table*}[t]
\footnotesize
%\vspace{-15pt}
  \centering
    \setlength{\abovecaptionskip}{2.5pt}
    \setlength{\belowcaptionskip}{-7.5pt}
  \caption{Typical examples of requirement description templates. Among these, the State-Change template is the most used, representing a state transition; the Bound-Check template indicates that the system must meet a certain boundary condition; and the Work-Mode-Change template represents a switch in the control system's operational mode. The red content in the requirement templates corresponds to the fillable fields, while the bold content in the TNL statements provides examples of how these fields are populated.}
  \resizebox{\textwidth}{!}{
    \begin{tabular}{lll}
    \toprule
    \rowcolor[rgb]{ .851,  .851,  .851} \textbf{S No.} & \textbf{Type} & \textbf{Requirement Templates and TNL Statements} \\
    \midrule
    \multirow{2}[2]{*}{1} & State & \textcolor{purple}{\textbf{Component}} shall always satisfy if ( \textcolor{purple}{\textbf{input\_state}} \& \textcolor{purple}{\textbf{condition}}) then next \textcolor{purple}{\textbf{output\_state}}. \\
          & Change   & 
          \textbf{`Communicator'} shall always satisfy if (\textbf{`signal\_lost'} \& \textbf{`mission\_phase'}) then next\textbf{`backup'}.
         \\
    \midrule
    \multirow{2}[2]{*}{2} & Bound & In \textcolor{purple}{\textbf{work\_mode}}, the \textcolor{purple}{\textbf{component}} shall always satisfy \textcolor{purple}{\textbf{bounds}}. \\
          & Check   & In \textbf{`pitch\_search mode'}, the \textbf{`gyroscope'} shall always satisfy \textbf{`roll\_target\_velocity = 0'}. \\
    \midrule
    \multirow{2}[2]{*}{3} & Work Mode & Upon ( \textcolor{purple}{\textbf{input\_work\_mode}} \& \textcolor{purple}{\textbf{condition}} ) \textcolor{purple}{\textbf{component}} shall at the next timepoint satisfy \textcolor{purple}{\textbf{output\_work\_mode}}. \\
          & Change   & Upon ( \textbf{`pitch\_search'} \& \textbf{`sun\_not\_found'} ) \textbf{`Spacecraft'} shall at the next timepoint satisfy \textbf{`roll\_search'}. \\

          % TNL   & Upon ( \textbf{`pitch\_search'} \& \textbf{`mode\_duration'} $\geq$ 720s \& \textbf{`sun\_not\_found'} ) \textbf{`Spacecraft'} shall at the next timepoint satisfy \textbf{`roll\_search'}. \\
    
    \midrule
    \multirow{2}[2]{*}{4} & Command & Upon \textcolor{purple}{\textbf{command}} the \textcolor{purple}{\textbf{component}} shall \textcolor{purple}{\textbf{timing}} satisfy \textcolor{purple}{\textbf{action}}. \\
          & Process   & Upon \textbf{`command\_opcode = 29'} the software shall \textbf{`immediately'} satisfy \textbf{`retract\_landing\_gear\_command'}. \\

    \midrule
    \multirow{2}[2]{*}{5} & State & 
    
    In \textcolor{purple}{\textbf{work mode}} the \textcolor{purple}{\textbf{component}} shall immediately satisfy if \textcolor{purple}{\textbf{condition}} then \textcolor{purple}{\textbf{response}}.
    
    \\
          & Response   & In \textbf{roll\_hold mode} the \textbf{`Spacecraft'} shall immediately satisfy if \textbf{`roll\_angle\_up'} then \textbf{`roll\_hold'}. \\

    \midrule
    \multirow{2}[2]{*}{6} & State & The \textcolor{purple}{\textbf{component}} shall maintain \textcolor{purple}{\textbf{state}} unless \textcolor{purple}{\textbf{condition}}. \\
          & Maintenance   & The \textbf{`alarm system'} shall maintain \textbf{`active'} unless \textbf{`system\_disabled'}. \\

    \midrule
    \rowcolor[rgb]{ .851,  .851,  .851} \multirow{1}[1]{*}{7} &$\dots\dots\dots$  &$\dots\dots\dots$
    
    \\
    \bottomrule
    \end{tabular}}
  \label{tab:templates_example}%
\end{table*}
\begin{table}[t]
%\vspace{-15pt}
\footnotesize
\setstretch{0.9}
    \centering
    \setlength\tabcolsep{10pt}
    \setlength{\abovecaptionskip}{2.5pt}
    \setlength{\belowcaptionskip}{-7.5pt}
    \caption{Statistics for Requirement Documents Used for Analysis and Testing}
    \begin{tabular}{lccc}
    \toprule
    \rowcolor[rgb]{ .851,  .851,  .851} \textbf{Category} & \begin{tabular}[c]{@{}c@{}}\textbf{Documents}\\ \textbf{Num}\end{tabular} & \begin{tabular}[c]{@{}c@{}}\textbf{Average}\\ \textbf{Word Count}\end{tabular} & \begin{tabular}[c]{@{}c@{}}\textbf{Requirement}\\ \textbf{Num}\end{tabular} \\
    \midrule
    Documents for Analysis & 8     & 2891  & 427 \\
    Documents for Testing & 1     & 3446  & 79 \\
    \bottomrule
    \end{tabular}
  \label{tab:doc_statistics}
  \vspace{-5pt}
\end{table}
